# Supplementary material for: Self-Calibrating, Fully Differentiable NLOS Inverse Rendering
Source: arXiv:2309.12047 source file (2023-09-26)
Supplement: Supplementary file 2 [file appendix.tex]

\appendix
\section{Appendix}
